# Supplementary material for: Complementary Frequency-Varying Awareness Network for Open-Set Fine-Grained Image Recognition
Source: arXiv:2307.07214 source file (2025-05-19)
Supplement: Supplementary file 1 [file supplementary_matrial_20221106.pdf]

# Supplementary Material for the Paper: Complementary Frequency-Varying Awareness Network for Open-Set Fine-Grained Image Recognition

Anonymous CVPR submission

Paper ID 2423

## A. Appendix

This appendix is organized as follows:

- Section A.1 introduces some preliminary information about the FAF (*i.e.*, the frequency-adjustable filter);
- Section A.2 gives more implementation details of the proposed CFAN-OSFGR method;
- Section A.3 provides additional experimental results. Firstly, Section A.3.1 provides the details of analyzing the influence of the values in the initial adjustable vectors $\boldsymbol{p}^h$ and $\boldsymbol{p}^l$ of the two sequences at the inference stage on the model performance. Next, Section A.3.2 shows additional results on the two coarse-grained datasets CIFAR+10/+50 [4, 5] and TinyImageNet [6]. Then, Section A.3.3 provides additional results of analyzing the influence of the size after upsampling. Next, Section A.3.4 exhibits additional results of analyzing the influence of the number of moments (also the length of the high- or low-frequency sequence, *i.e.*, $N_f$). Last, Section A.3.5 shows additional results of analyzing the influence of operation position of the complementary frequency-varying awareness mechanism in the SwinB [8] backbone.

### A.1. Preliminaries on the FAF

The designed frequency-adjustable filter (FAF) is based on the exponential power (EP) function, which is also called the generalized Gaussian function and can represent sub-Gaussian and super-Gaussian functions in addition to the Gaussian function [1,2,9]. According to the parametric form suggested in [2], the complete form of the EP function is formulated as:

$$f = \frac{1}{2\sigma p^{\frac{1}{p}}\Gamma(1+\frac{1}{p})} e^{-\frac{|m-\mu|^p}{p\sigma^p}} \tag{A.1}$$

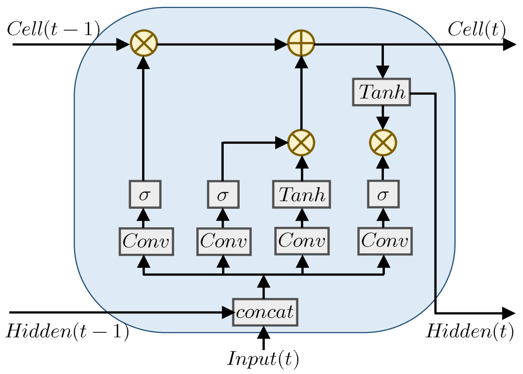


Figure A.1. Architecture of the LSTM unit at each moment. The '$Conv$', '$\sigma$', '$Tanh$' represent the convolutional block, Sigmoid layer and Tanh layer, respectively.

where $m$ is the argument, $\Gamma(\cdot)$ is the Gamma function, and $\{\mu, \sigma, p\}$ $(\sigma > 0, p > 0)$ is a group of parameters controlling the position, scale and shape of the EP function respectively. The shape parameter $p$ is adjustable in the EP function but fixed to 2 in the Gaussian function, which endows the EP function with flexibility. In order to limit the values in FAF within the range of $(0, 1)$, we discard the coefficient part before the exponential power part.

### A.2. Implementation Details

#### A.2.1 Details of the LSTMs

The network architectures of the two LSTMs are the same, whose unit at each moment is shown in Fig. A.1 and the network function $LSTM(\cdot)$ is detailed as follows:

$$\begin{aligned} &\boldsymbol{H}_t \leftarrow [\boldsymbol{H}_{t-1}; \boldsymbol{x}^t]; \\ &\boldsymbol{C}_t \leftarrow \boldsymbol{C}_{t-1} * \sigma(Conv(\boldsymbol{H}_t)) + \\ &\qquad \sigma(Conv(\boldsymbol{H}_t)) * Tanh(Conv(\boldsymbol{H}_t)); \\ &\boldsymbol{H}_t \leftarrow Tanh(\boldsymbol{C}_t) * \sigma(Conv(\boldsymbol{H}_t)); \end{aligned} \tag{A.2}$$

Table A.1. The numbers of known/unknown classes used in the experiments.

| Fine/Coarse-grained | Setting | Dataset | Known | Unknown | | |
|---|---|---|---|---|---|---|
| Fine-grained | Standard-dataset | CUB | 100 | Easy | Medium | Hard |
| | | | | 32 | 34 | 34 |
| | | Aircraft | 50 | Easy | Medium | Hard |
| | | | | 20 | 17 | 13 |
| | | Stanford-Cars | 98 | 98 | | |
| | Cross-dataset | CUB<br>Stanford-Cars | 50<br>50 | 200<br>196 | | |
| Coarse-grained | - | CIFAR+10/+50 | 10 | 10/50 | | |
| | | TinyImageNet | 20 | 180 | | |

Table A.2. OSFGR results on CUB under the *standard-dataset setting* of the proposed CFAN-OSFGR with different values in the initial adjustable vectors $\boldsymbol{p}^h$ and $\boldsymbol{p}^l$ of the high- and low-frequency sequences at the inference stage.

| $p$ values | ACC | AUROC (Easy/Medium/Hard) | OSCR (Easy/Medium/Hard) |
|---|---|---|---|
| 0.21 | 0.947 | 0.955/0.909/0.827 | 0.916/0.878/0.804 |
| 0.5 | 0.947 | 0.954/0.909/0.832 | 0.915/0.878/0.809 |
| 1 | 0.947 | 0.954/0.909/0.833 | 0.915/0.877/0.810 |
| 3 | 0.947 | 0.954/0.909/0.834 | 0.915/0.877/0.811 |
| 5 | 0.947 | 0.954/0.909/0.834 | 0.915/0.877/0.811 |
| 10 | 0.947 | 0.954/0.909/0.833 | 0.916/0.877/0.811 |
| 15 | 0.948 | 0.954/0.908/0.833 | 0.916/0.878/0.811 |
| 19.9 | 0.948 | 0.954/0.908/0.833 | 0.916/0.877/0.811 |

Table A.3. OSFGR results on Aircraft under the *standard-dataset setting* of the proposed CFAN-OSFGR with different values in the initial adjustable vectors $\boldsymbol{p}^h$ and $\boldsymbol{p}^l$ of the high- and low-frequency sequences at the inference stage.

| $p$ values | ACC | AUROC (Easy/Medium/Hard) | OSCR (Easy/Medium/Hard) |
|---|---|---|---|
| 0.21 | 0.916 | 0.915/0.892/0.833 | 0.865/0.845/0.798 |
| 0.5 | 0.917 | 0.914/0.892/0.838 | 0.865/0.845/0.802 |
| 1 | 0.917 | 0.913/0.892/0.839 | 0.864/0.845/0.803 |
| 3 | 0.917 | 0.913/0.892/0.839 | 0.864/0.845/0.803 |
| 5 | 0.917 | 0.913/0.892/0.839 | 0.864/0.845/0.803 |
| 10 | 0.917 | 0.913/0.892/0.839 | 0.864/0.845/0.803 |
| 15 | 0.917 | 0.913/0.892/0.839 | 0.864/0.845/0.803 |
| 19.9 | 0.917 | 0.913/0.892/0.839 | 0.864/0.845/0.803 |

where $Conv$ is detailed as follows:

```
Conv2d(in=2*128,out=64,k=3,s=1,p=1);
BatchNorm2d(64);
ReLU();
Conv2d(in=64,out=128,k=3,s=1,p=1);
BatchNorm2d(128).
```

#### A.2.2 Details of the Number of Known/Unknown Classes

Table A.1 shows the number of the split known/unknown classes from the two dataset settings (*i.e.*, the *standard-dataset setting* and the *cross-dataset setting*) on both fine-grained and coarse-grained datasets.

## A.3. Additional Results

### A.3.1 Influence of the Initial Values in the Adjustable Vectors in Testing

Here, we conduct an experiment for analyzing the influence of different values in the two initial adjustable vectors $\boldsymbol{p}^h$ and $\boldsymbol{p}^l$ of the high- and low-frequency sequences at the inference stage on the model performance. Specifically, we test the model with all values in the two vectors fixed to $\{0.21, 0.5, 1, 3, 5, 10, 15, 19.9\}$ respectively. The corresponding OSFGR results on the three fine-grained datasets (*i.e.*, CUB [12], Aircraft [10] and Stanford-Cars [3]) under the *standard-dataset setting* are reported in Tables A.2, A.3 and A.4, respectively. As seen from these tables, the result-

Table A.4. OSFGR results on Stanford-Cars under the *standard-dataset setting* of the proposed CFAN-OSFGR with different values in the initial adjustable vectors $\boldsymbol{p}^h$ and $\boldsymbol{p}^l$ of the high- and low-frequency sequences at the inference stage.

| $p$ values | ACC | AUROC | OSCR |
|---|---|---|---|
| 0.21 | 0.895 | 0.939 | 0.859 |
| 0.5 | 0.896 | 0.939 | 0.859 |
| 1 | 0.896 | 0.939 | 0.859 |
| 3 | 0.896 | 0.939 | 0.859 |
| 5 | 0.896 | 0.939 | 0.859 |
| 10 | 0.895 | 0.939 | 0.859 |
| 15 | 0.895 | 0.939 | 0.859 |
| 19.9 | 0.895 | 0.939 | 0.859 |

Table A.5. Comparison of ACC, AUROC and OSCR results on CUB under the *standard-dataset setting* of the proposed CFAN-OSFGR method with different feature map sizes after upsampling.

| Backbone | Method | ACC | AUROC (Easy/Medium/Hard) | OSCR (Easy/Medium/Hard) |
|---|---|---|---|---|
| CNN | OpenHybrid | 0.683 | 0.873/0.862/0.739 | 0.662/0.649/0.531 |
| | OpenGAN | 0.799 | 0.801/0.765/0.707 | 0.725/0.706/0.648 |
| | ARPL | 0.863 | 0.814/0.772/0.703 | 0.747/0.710/0.659 |
| | GCPL | 0.783 | 0.805/0.732/0.645 | 0.711/0.619/0.565 |
| | GMVAE-OSR | 0.725 | 0.826/0.750/0.704 | 0.694/0.628/0.553 |
| | CAMV | 0.836 | 0.845/0.802/0.709 | 0.746/0.715/0.640 |
| | Cross-Entropy+ | 0.862 | 0.883/0.823/0.763 | 0.798/0.754/0.708 |
| SwinB | Backbone | 0.949 | 0.945/0.875/0.804 | 0.908/0.848/0.781 |
| | OpenHybrid | 0.950 | 0.953/0.881/0.808 | 0.918/0.855/0.783 |
| | ARPL | 0.952 | 0.948/0.877/0.810 | 0.912/0.850/0.788 |
| | Cross-Entropy+ | **0.953** | 0.950/0.879/0.815 | 0.917/0.854/0.794 |
| | Trans-AUG | 0.950 | 0.953/0.882/0.818 | 0.914/0.854/0.795 |
| | MoEP-AE-OSR | 0.948 | 0.957/0.889/0.814 | 0.915/0.856/0.787 |
| | CFAN-OSFGR (w/o upsampling) | 0.946 | 0.959/0.910/0.828 | 0.918/0.879/0.805 |
| | CFAN-OSFGR (2-times upsampling) | 0.948 | **0.964/0.912/0.842** | **0.924/0.881/0.819** |
| | CFAN-OSFGR (4-times upsampling) | 0.947 | 0.954/0.909/0.833 | 0.915/0.877/0.810 |
| | CFAN-OSFGR (8-times upsampling) | 0.948 | 0.951/0.887/0.836 | 0.914/0.859/0.814 |

Table A.6. Detailed OSR results on CIFAR+10/+50 of the proposed CFAN-OSFGR.

| trial | AUROC | ACC |
|---|---|---|
| 0 | 0.988/0.983 | 0.988 |
| 1 | 0.995/0.993 | 0.990 |
| 2 | 0.994/0.993 | 0.990 |
| 3 | 0.996/0.992 | 0.990 |
| 4 | 0.996/0.994 | 0.991 |
| Avg | 0.994/0.991 | 0.990 |

Table A.7. Detailed OSR results on TinyImageNet of the proposed CFAN-OSFGR.

| trial | AUROC | ACC |
|---|---|---|
| 0 | 0.960 | 0.957 |
| 1 | 0.950 | 0.966 |
| 2 | 0.957 | 0.962 |
| 3 | 0.960 | 0.967 |
| 4 | 0.950 | 0.961 |
| Avg | 0.955 | 0.963 |

s vary very slightly when these values vary in $[0.21, 19.9]$, demonstrating that the CFAN-OSFGR model is robust to different values in the initial adjustable vectors of the two sequences at the inference stage.

### A.3.2 Detailed Results on Coarse-Grained Datasets

Most of the existing OSR methods are evaluated on 5 coarse-grained datasets (MNIST [7], SVHN [11], CIFAR10 [5], CIFAR+10/+50 [4,5] and TinyImageNet [6]) in their original papers. Among these datasets, the CIFAR+10/+50 and TinyImageNet are the most complex and challenging, which we use for evaluating the model performance on the coarse-grained datasets. Specifically, the results are averaged over 5 same trials as used in most OSR methods, and the detailed results on CIFAR+10/+50 and TinyImageNet are reported in Tables A.6 and A.7, respectively.

### A.3.3 Influence of the Size After Upsampling

Considering the feature map obtained from the feature extraction module (SwinB [8] is directly used here) is relatively small, we conduct upsampling on the feature map for better filtering in the frequency domain and pruning the channels of the feature map for avoiding the undesired model complexity. Specifically, the feature maps are 4-times upsampled in our experiments. Here, we conduct an experiment for analyzing the influence of the size after sampling on the model performance on CUB under the *standard-dataset setting*, and the results are reported in Table A.5, where the results of the 12 state-of-the-art OSR/OSFGR comparative methods are also listed for better comparison.

Two points can be seen from this table:

(1) The proposed CFAN-OSFGR method with different sizes after upsampling still outperforms the 12 existing state-of-the-art OSR/OSFGR methods under the AUROC and OSCR metrics in most cases, demonstrating the effectiveness of CFAN-OSFGR without regard to the feature map size after upsampling.

(2) Besides, the results under the AUROC and OSCR metrics of CFAN-OSFGR with different feature map sizes vary in $[1\%, 2.5\%]$, indicating that the feature map size does affect the model performance to some extent. Moreover, the proposed method with 2-times upsampling achieves better results than larger sizes after upsampling, indicating that the upsampling operation maybe sometimes helpful for improving the model performance but cannot provide promising improvement.

### A.3.4 Influence of the Number of Moments

We also conduct an ablation experiment for analyzing the influence of the number of moments $N_f$ on the model performance, the OSFGR results on CUB under the *standard-*

Table A.8. OSFGR results on CUB under the *standard-dataset setting* of the proposed CFAN-OSFGR with different $N_f$.

| $N_f$ | ACC | AUROC (Easy/Medium/Hard) | OSCR (Easy/Medium/Hard) |
|---|---|---|---|
| 1 | 0.945 | 0.947/0.884/0.812 | 0.909/0.853/0.782 |
| 2 | 0.944 | 0.945/0.897/0.828 | 0.902/0.864/0.796 |
| 4 | 0.947 | 0.954/0.909/0.833 | 0.915/0.877/0.810 |
| 6 | 0.946 | 0.955/0.913/0.835 | 0.913/0.882/0.817 |
| 8 | 0.947 | 0.950/0.917/0.834 | 0.912/0.883/0.815 |

Table A.9. OSFGR results on CUB under the *standard-dataset setting* of the proposed CFAN-OSFGR operated on different blocks of SwinB.

| Operation Block | ACC | AUROC (Easy/Medium/Hard) | OSCR (Easy/Medium/Hard) |
|---|---|---|---|
| Block1 | 0.933 | 0.946/0.888/0.789 | 0.897/0.850/0.762 |
| Block2 | 0.933 | 0.941/0.894/0.781 | 0.893/0.855/0.754 |
| Block3 | 0.944 | 0.949/0.897/0.824 | 0.910/0.867/0.802 |
| Block4 | 0.947 | 0.954/0.909/0.833 | 0.915/0.877/0.810 |

*dataset setting* are reported in Table A.8. As seen from this table, more moments usually lead to better results when $N_f$ varies in $[1, 6]$, but a too large $N_f$ (*e.g.*, $N_f = 8$) is unable to further improve the model performance.

#### A.3.5 Influence of the Operation Position

Considering that the preliminary feature is obtained from the final block of the feature extraction module, we additionally conduct an experiment on CUB under the *standard-dataset setting* for investigating the influence of the operation position of the complementary frequency-varying awareness mechanism. Specifically, the mechanism is operated on the four blocks (*i.e.*, Block1, Block2, Block3 and Block4, the discriminability of the features outputted from these blocks increases progressively) of the SwinB respectively, and the corresponding results are reported in Table A.9. As seen from this table, the results on Block3 and Block4 are better than those on Block1 and Block2, and the results on Block4 are better than those on Block3. These results indicate that a more discriminative preliminary feature is helpful for improving the model performance. Hence, applying the proposed CFAN-OSFGR mechanism at the end of a backbone network is more suitable for the OSFGR task.

## References

[1] G. Agró. Maximum likelihood estimation for the exponential power function parameters. *Communications in Statistics-Simulation and Computation*, 24(2):523–536, 1995. 1

[2] Christian Kleiber and Samuel Kotza. *Statistical Size Distributions in Economics and Actuarial Sciences*. John Wiley & Sons, 2003. 1

[3] Jonathan Krause, Michael Stark, Jia Deng, and Li Fei-Fei. 3d object representations for fine-grained categorization. In *IEEE International Conference on Computer Vision*, 2013. 2

[4] Alex Krizhevsky. Learning multiple layers of features from tiny images, 2009. *Technical report*. 1, 3

[5] Alex Krizhevsky and Geoffrey Hinton. Convolutional deep belief networks on cifar-10, 2010. *Technical report*. 1, 3

[6] Ya Le and Xuan Yang. Tiny imagenet visual recognition challenge, 2015. *CS 231N*. 1, 3

[7] Yann LeCun, Corinna Cortes, and Christopher J.C. Burges. The mnist database of handwritten digits. 3

[8] Ze Liu, Yutong Lin, Yue Cao, Han Hu, Yixuan Wei, Zheng Zhang, Stephen Lin, and Baining Guo. Swin transformer: Hierarchical vision transformer using shifted windows. In *IEEE International Conference on Computer Vision*, 2021. 1, 3

[9] R. Duncan Luce. Reduction invariance and prelec's weighting functions. *Journal of Mathematical Psychology*, 45(1):167–179, 2001. 1

[10] Subhransu Maji, Esa Rahtu, Juho Kannala, Matthew Blaschko, and Andrea Vedaldi. Fine-grained visual classification of aircraft. *arXiv preprint. arXiv:1306.5151*, 2013. 2

[11] Yuval Netzer, Tao Wang, Adam Coates, Alessandro Bissacco, Bo Wu, and Andrew Y. Ng. Reading digits in natural images with unsupervised feature learning. In *Conference and Workshop on Neural Information Processing Systems*. 3

[12] Catherine Wah, Steve Branson, Peter Welinder, Pietro Perona, and Serge Belongie. The CaltechUCSD Birds-200-2011 Dataset. Technical report, California Institute of Technology, 2011. 2
