# Supplementary material for: Complementary Frequency-Varying Awareness Network for Open-Set Fine-Grained Image Recognition
Source: arXiv:2307.07214 source file (2025-05-19)
Supplement: Supplementary file 3 [file supplementary_matrial_20221112.pdf]

# Supplementary Material for the Paper: Complementary Frequency-Varying Awareness Network for Open-Set Fine-Grained Image Recognition

Anonymous CVPR submission

Paper ID 2423

## 不是附录 A. Appendix ABC

This appendix is organized as follows:

- Section A.1 gives more implementation details of the proposed CFAN-OSFGR method;
- Section A.2 provides additional experimental results. Firstly, Section A.2.1 provides the details of analyzing the influence of the values in the initial adjustable vectors  $p_h^1$  and  $p_l^1$  of the two time series at the inference stage on the model performance. Next, Section A.2.2 shows additional results on the two coarse-grained datasets CIFAR+10/+50 [2, 3] and TinyImageNet [4]. Then, Section A.2.3 provides additional results of analyzing the influence of the feature map size after upsampling. Next, Section A.2.4 shows additional results of analyzing the influence of the number of moments (also the length of the high- or low-frequency time series, *i.e.*,  $N_f$ ). Lastly, Section A.2.5 shows additional results of analyzing the influence of different blocks in the feature extraction module.

### A.1. Implementation Details

#### A.2.1 Details of the LSTMs

The network architectures of the two LSTMs in the C-TA module (*i.e.*, the complementary temporal aggregation module) are the same, whose unit at each moment is shown in Fig. A.1 and the network function (taking  $LSTM_h(\cdot)$  as an example) is detailed as follows:

$$\begin{aligned} H_h^t &\leftarrow [H_h^{t-1}; X_h^t]; \\ C_h^t &\leftarrow C_h^{t-1} * \sigma(Conv(H_h^t)) + \\ &\quad \sigma(Conv(H_h^t)) * Tanh(Conv(H_h^t)); \\ H_h^t &\leftarrow Tanh(C_h^t) * \sigma(Conv(H_h^t)); \end{aligned} \quad (A.1)$$

where  $Conv$  is detailed as follows:

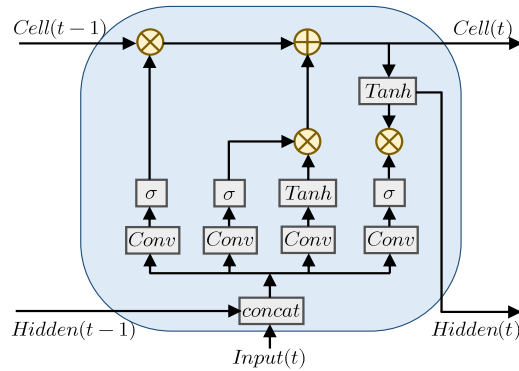

Figure A.1. Architecture of the LSTM unit at each moment. The ‘Conv’, ‘σ’, ‘Tanh’ represent the convolutional block, Sigmoid layer, and Tanh layer, respectively.

```
Conv2d(in=2*128, out=64, k=3, s=1, p=1);
BatchNorm2d(64);
ReLU();
Conv2d(in=64, out=128, k=3, s=1, p=1);
BatchNorm2d(128);
```

#### A.2.2 Details of the Number of Known/Unknown Classes

Table A.1 summarizes the number of the split known/unknown classes from the two dataset settings (*i.e.*, the *standard-dataset setting* and the *cross-dataset setting*) on both fine-grained and coarse-grained datasets.

### A.2. Additional Results

#### A.2.1 Influence of the Values in the Initial Adjustable

Vectors in Testing

Here, we conduct an experiment for analyzing the influence of different values in the two initial adjustable vectors  $p_h^1$  and  $p_l^1$  of the high- and low-frequency time series at the inference stage on the model performance. Specifically, we test the model with all values in the two vectors fixed to  $\{0.2, 0.5, 1, 3, 5, 10, 15, 20\}$  respectively. The corresponding OSFGR results on the three fine-grained datasets (*i.e.*,

多次随机，计算均值和标准差（括号里）  
只做CUB就行

由表中看出，标准差很小，不敏感

定冠词可以去掉

Table A.1. The numbers of known/unknown classes used in the experiments.

| Fine/Coarse-grained | Setting          | Dataset       | Known | Unknown |        |      |
|---------------------|------------------|---------------|-------|---------|--------|------|
| Fine-grained        | Standard-dataset | CUB           | 100   | Easy    | Medium | Hard |
|                     |                  |               |       | 32      | 34     | 34   |
|                     |                  | Aircraft      | 50    | Easy    | Medium | Hard |
|                     |                  |               |       | 20      | 17     | 13   |
|                     | Cross-dataset    | Stanford-Cars | 98    | 98      |        |      |
|                     |                  | CUB           | 50    | 200     |        |      |
|                     |                  | Stanford-Cars | 50    | 196     |        |      |
| CIFAR+10/+50        |                  | 10            | 10/50 |         |        |      |
| Coarse-grained      | -                | TinyImageNet  | 20    | 180     |        |      |

句子太长了，先进行删减，然后进行短语调整，或者加些逗号。

Table A.2. OSFGR results on CUB under the *standard-dataset setting* of the proposed CFAN-OSFGR method with different values in the initial adjustable vectors  $p_h^1$  and  $p_l^1$  of the high- and low-frequency time series at the inference stage.

| $p$ values | ACC   | AUROC              | OSCR               |
|------------|-------|--------------------|--------------------|
|            |       | (Easy/Medium/Hard) | (Easy/Medium/Hard) |
| 0.2        | 0.947 | 0.955/0.909/0.827  | 0.916/0.878/0.804  |
| 0.5        | 0.947 | 0.954/0.909/0.832  | 0.915/0.878/0.809  |
| 1          | 0.947 | 0.954/0.909/0.833  | 0.915/0.877/0.810  |
| 3          | 0.947 | 0.954/0.909/0.834  | 0.915/0.877/0.811  |
| 5          | 0.947 | 0.954/0.909/0.834  | 0.915/0.877/0.811  |
| 10         | 0.947 | 0.954/0.909/0.833  | 0.916/0.877/0.811  |
| 15         | 0.948 | 0.954/0.908/0.833  | 0.916/0.878/0.811  |
| 20         | 0.948 | 0.954/0.908/0.833  | 0.916/0.877/0.811  |

Table A.3. OSFGR results on Aircraft under the *standard-dataset setting* of the proposed CFAN-OSFGR method with different values in the initial adjustable vectors  $p_h^1$  and  $p_l^1$  of the high- and low-frequency time series at the inference stage.

| $p$ values | ACC   | AUROC              | OSCR               |
|------------|-------|--------------------|--------------------|
|            |       | (Easy/Medium/Hard) | (Easy/Medium/Hard) |
| 0.2        | 0.916 | 0.915/0.892/0.833  | 0.865/0.845/0.798  |
| 0.5        | 0.917 | 0.914/0.892/0.838  | 0.865/0.845/0.802  |
| 1          | 0.917 | 0.913/0.892/0.839  | 0.864/0.845/0.803  |
| 3          | 0.917 | 0.913/0.892/0.839  | 0.864/0.845/0.803  |
| 5          | 0.917 | 0.913/0.892/0.839  | 0.864/0.845/0.803  |
| 10         | 0.917 | 0.913/0.892/0.839  | 0.864/0.845/0.803  |
| 15         | 0.917 | 0.913/0.892/0.839  | 0.864/0.845/0.803  |
| 20         | 0.917 | 0.913/0.892/0.839  | 0.864/0.845/0.803  |

Table A.4. OSFGR results on Stanford-Cars under the *standard-dataset setting* of the proposed CFAN-OSFGR method with different values in the initial adjustable vectors  $p_h^1$  and  $p_l^1$  of the high- and low-frequency time series at the inference stage.

| $p$ values | ACC   | AUROC | OSCR  |
|------------|-------|-------|-------|
| 0.2        | 0.895 | 0.939 | 0.859 |
| 0.5        | 0.896 | 0.939 | 0.859 |
| 1          | 0.896 | 0.939 | 0.859 |
| 3          | 0.896 | 0.939 | 0.859 |
| 5          | 0.896 | 0.939 | 0.859 |
| 10         | 0.895 | 0.939 | 0.859 |
| 15         | 0.895 | 0.939 | 0.859 |
| 20         | 0.895 | 0.939 | 0.859 |

CUB [9], Aircraft [7], and Stanford-Cars [1]) under the *standard-dataset setting* are reported in Tables A.2, A.3, and A.4, respectively. As seen from these tables, the results vary very slightly when these values vary in [0.2, 20], demonstrating that the CFAN-OSFGR model is robust to different values in the initial adjustable vectors  $p_h^1$  and  $p_l^1$  of the high- and low-frequency time series at the inference stage.

Table A.5. Detailed OSR results on CIFAR+10/+50 of the proposed CFAN-OSFGR method.

| trial | AUROC       | ACC   |
|-------|-------------|-------|
| 0     | 0.988/0.983 | 0.988 |
| 1     | 0.995/0.993 | 0.990 |
| 2     | 0.994/0.993 | 0.990 |
| 3     | 0.996/0.992 | 0.990 |
| 4     | 0.996/0.994 | 0.991 |
| Avg   | 0.994/0.991 | 0.990 |

Table A.6. Detailed OSR results on TinyImageNet of the proposed CFAN-OSFGR method.

| trial | AUROC | ACC   |
|-------|-------|-------|
| 0     | 0.960 | 0.957 |
| 1     | 0.950 | 0.966 |
| 2     | 0.957 | 0.962 |
| 3     | 0.960 | 0.967 |
| 4     | 0.950 | 0.961 |
| Avg   | 0.955 | 0.963 |

A.2.2 Detailed Results on Coarse-Grained Datasets

Most of the existing OSR methods are evaluated on 5 coarse-grained datasets (MNIST [5], SVHN [8], CIFAR10  
在正文中报道是平均值

Table A.7. Comparison of ACC, AUROC, and OSCR results on CUB under the *standard-dataset setting* of the proposed CFAN-OSFGR method with different feature map sizes after upsampling.

| Backbone | Method                          | ACC          | AUROC<br>(Easy/Medium/Hard) | OSCR<br>(Easy/Medium/Hard) |
|----------|---------------------------------|--------------|-----------------------------|----------------------------|
| CNN      | OpenHybrid                      | 0.683        | 0.873/0.862/0.739           | 0.662/0.649/0.531          |
|          | OpenGAN                         | 0.799        | 0.801/0.765/0.707           | 0.725/0.706/0.648          |
|          | ARPL                            | 0.863        | 0.814/0.772/0.703           | 0.747/0.710/0.659          |
|          | GCPL                            | 0.783        | 0.805/0.732/0.645           | 0.711/0.619/0.565          |
|          | GMVAE-OSR                       | 0.725        | 0.826/0.750/0.704           | 0.694/0.628/0.553          |
|          | CAMV                            | 0.836        | 0.845/0.802/0.709           | 0.746/0.715/0.640          |
|          | Cross-Entropy+                  | 0.862        | 0.883/0.823/0.763           | 0.798/0.754/0.708          |
| SwinB    | Backbone                        | 0.949        | 0.945/0.875/0.804           | 0.908/0.848/0.781          |
|          | OpenHybrid                      | 0.950        | 0.953/0.881/0.808           | 0.918/0.855/0.783          |
|          | ARPL                            | 0.952        | 0.948/0.877/0.810           | 0.912/0.850/0.788          |
|          | Cross-Entropy+                  | <b>0.953</b> | 0.950/0.879/0.815           | 0.917/0.854/0.794          |
|          | Trans-AUG                       | 0.950        | 0.953/0.882/0.818           | 0.914/0.854/0.795          |
|          | MoEP-AE-OSR                     | 0.948        | 0.957/0.889/0.814           | 0.915/0.856/0.787          |
|          | CFAN-OSFGR (w/o upsampling)     | 0.946        | 0.959/0.910/0.828           | 0.918/0.879/0.805          |
|          | CFAN-OSFGR (2-times upsampling) | 0.948        | <b>0.964/0.912/0.842</b>    | <b>0.924/0.881/0.819</b>   |
|          | CFAN-OSFGR (4-times upsampling) | 0.947        | 0.954/0.909/0.833           | 0.915/0.877/0.810          |
|          | CFAN-OSFGR (8-times upsampling) | 0.948        | 0.951/0.887/0.836           | 0.914/0.859/0.814          |

Table A.8. OSFGR results on CUB under the *standard-dataset setting* of the proposed CFAN-OSFGR method with different  $N_f$ .

| $N_f$ | ACC   | AUROC<br>(Easy/Medium/Hard) | OSCR<br>(Easy/Medium/Hard) |
|-------|-------|-----------------------------|----------------------------|
| 1     | 0.945 | 0.947/0.884/0.812           | 0.909/0.853/0.782          |
| 2     | 0.944 | 0.945/0.897/0.828           | 0.902/0.864/0.796          |
| 4     | 0.947 | 0.954/0.909/0.833           | 0.915/0.877/0.810          |
| 6     | 0.946 | 0.955/0.913/0.835           | 0.913/0.882/0.817          |
| 8     | 0.947 | 0.950/0.917/0.834           | 0.912/0.883/0.815          |

Table A.9. OSFGR results on CUB under the *standard-dataset setting* of the proposed CFAN-OSFGR method with the preliminary features extracted from different blocks of the SwinB backbone.

| Block  | ACC   | AUROC<br>(Easy/Medium/Hard) | OSCR<br>(Easy/Medium/Hard) |
|--------|-------|-----------------------------|----------------------------|
| Block1 | 0.933 | 0.946/0.888/0.789           | 0.897/0.850/0.762          |
| Block2 | 0.933 | 0.941/0.894/0.781           | 0.893/0.855/0.754          |
| Block3 | 0.944 | 0.949/0.897/0.824           | 0.910/0.867/0.802          |
| Block4 | 0.947 | 0.954/0.909/0.833           | 0.915/0.877/0.810          |

[3], CIFAR+10/+50 [2, 3] and TinyImageNet [4]) in their original papers. Among these datasets, the CIFAR+10/+50 and TinyImageNet are the most complex and challenging datasets, which we use for evaluating the model performance on the coarse-grained datasets. Specifically, the results are averaged over 5 same trials as used in most OSR methods, and the detailed results on CIFAR+10/+50 and TinyImageNet are reported in Tables A.5 and A.6, respectively.

### A.2.3 Influence of the Size After Upsampling

Considering the feature map obtained from the feature extraction module (SwinB [6] is directly used here) is relatively small, we conduct upsampling on the feature map for better filtering in the frequency domain, and simultaneously prune the channels of the feature map for decreasing the undesired model complexity. Specifically, the feature maps are 4-times upsampled in our experiments. Here, we con-

duct an experiment for analyzing the influence of the size after sampling on the model performance on CUB under the *standard-dataset setting* by training additional models with the upsampling size varying within  $\{1, 2, 8\}$  times respectively, whose results are reported in Table A.7, where the results of the 9 state-of-the-art OSR/OSFGR comparative methods are also listed for better comparison.

Two points can be seen from this table:

(1) The proposed CFAN-OSFGR method with different sizes after upsampling still outperforms the 9 existing state-of-the-art OSR/OSFGR methods under the AUROC and OSCR metrics in most cases, demonstrating the effectiveness of CFAN-OSFGR without regard to the feature map size after upsampling.

(2) Besides, the results under the AUROC and OSCR metrics vary within  $[1\%, 2.5\%]$  among the CFAN-OSFGR models with different feature map sizes, indicating that the feature map size does affect the model performance to some extent. Moreover, the proposed method with 2-times up-

sampling achieves better results than larger sizes after up-sampling as well as without upsampling, indicating that the upsampling operation may sometimes be helpful for improving the model performance but cannot provide promising improvement.

#### A.2.4 Influence of the Number of Moments

We also conduct an experiment for analyzing the influence of the number of moments  $N_f$  on the model performance. Specifically, we train models based on the proposed CFAN-OSFGR method with the value of  $N_f$  varying in  $\{1, 2, 6, 8\}$ , whose OSFGR results on CUB under the *standard-dataset setting* are reported in Table A.8. As seen from this table, a larger  $N_f$  usually leads to better results when  $N_f$  varies in  $[1, 6]$ , however, a too large  $N_f$  (e.g.,  $N_f = 8$ ) is unable to further improve the model performance.

#### ~~A.2.5 Influence of Different Blocks in the Feature Extraction Module~~

Considering that the preliminary feature is obtained from the final block of the feature extraction module, we additionally conduct an experiment on CUB under the *standard-dataset setting* for investigating the influence of different blocks in this module. Specifically, the preliminary features are extracted from the four blocks (i.e., Block1, Block2, Block3, and Block4, the discriminability of the features outputted from these blocks increases progressively) of the SwinB backbone respectively, and the corresponding results are reported in Table A.9. As seen from this table, the results on Block3 and Block4 are better than those on Block1 and Block2, and the results on Block4 are better than those on Block3. These results indicate that higher discriminability of the preliminary features is helpful for improving the model performance.

## References

[1] Jonathan Krause, Michael Stark, Jia Deng, and Li Fei-Fei. 3d object representations for fine-grained categorization. In *IEEE International Conference on Computer Vision*, 2013. 2

[2] Alex Krizhevsky. Learning multiple layers of features from tiny images, 2009. *Technical report*. 1, 3

[3] Alex Krizhevsky and Geoffrey Hinton. Convolutional deep belief networks on cifar-10, 2010. *Technical report*. 1, 3

[4] Ya Le and Xuan Yang. Tiny imagenet visual recognition challenge, 2015. *CS 231N*. 1, 3

[5] Yann LeCun, Corinna Cortes, and Christopher J.C. Burges. The mnist database of handwritten digits. 2

[6] Ze Liu, Yutong Lin, Yue Cao, Han Hu, Yixuan Wei, Zheng Zhang, Stephen Lin, and Baining Guo. Swin transformer: Hierarchical vision transformer using shifted windows. In *IEEE International Conference on Computer Vision*, 2021. 3

[7] Subhransu Maji, Esa Rahtu, Juho Kannala, Matthew Blaschko, and Andrea Vedaldi. Fine-grained visual classification of aircraft. *arXiv preprint. arXiv:1306.5151*, 2013. 2

[8] Yuval Netzer, Tao Wang, Adam Coates, Alessandro Bissacco, Bo Wu, and Andrew Y. Ng. Reading digits in natural images with unsupervised feature learning. In *Conference and Workshop on Neural Information Processing Systems*. 2

[9] Catherine Wah, Steve Branson, Peter Welinder, Pietro Perona, and Serge Belongie. The CaltechUCSD Birds-200-2011 Dataset. Technical report, California Institute of Technology, 2011. 2
